# Supplementary material for: PAIR-Diffusion: A Comprehensive Multimodal Object-Level Image Editor
Source: arXiv:2303.17546 source file (2024-04-08)
Supplement: Supplementary file 1 [file global.tex]

\begin{table*}
    \centering
    
    \footnotesize
    \resizebox{\linewidth}{!}{
    \setlength\tabcolsep{0.2pt}
    \begin{tabular}{cccccc}
            \includegraphics[trim=0 0 0 0,clip,width=0.2\columnwidth]{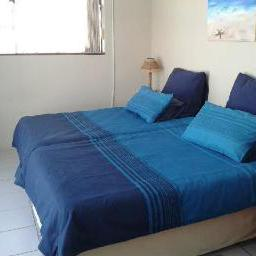} &
            \includegraphics[trim=0 0 0 0,clip,width=0.2\columnwidth]{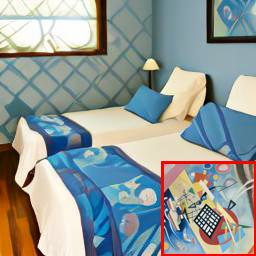} &
            \includegraphics[trim=0 0 0 0,clip,width=0.2\columnwidth]{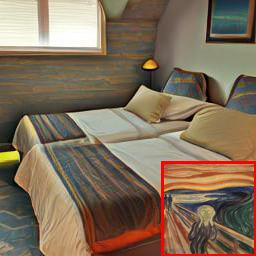} &
            \includegraphics[trim=0 0 0 0,clip,width=0.2\columnwidth]{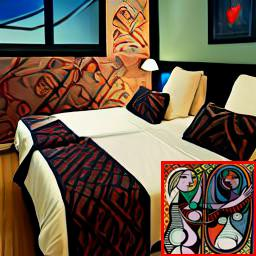} &
            \includegraphics[trim=0 0 0 0,clip,width=0.2\columnwidth]{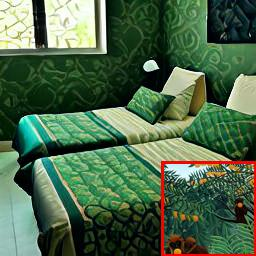} &
            \includegraphics[trim=0 0 0 0,clip,width=0.2\columnwidth]{supp/supp_qualitatives/od_global/images/bed/017.jpg} \\

            \includegraphics[trim=0 0 0 0,clip,width=0.2\columnwidth]{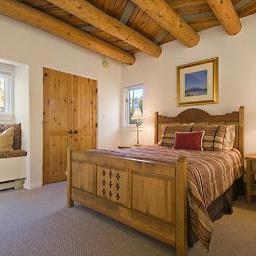} &
            \includegraphics[trim=0 0 0 0,clip,width=0.2\columnwidth]{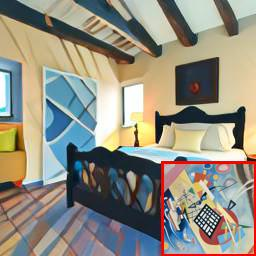} &
            \includegraphics[trim=0 0 0 0,clip,width=0.2\columnwidth]{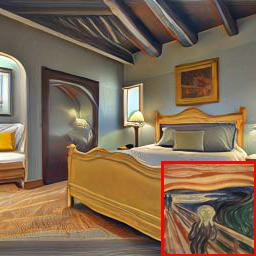} &
            \includegraphics[trim=0 0 0 0,clip,width=0.2\columnwidth]{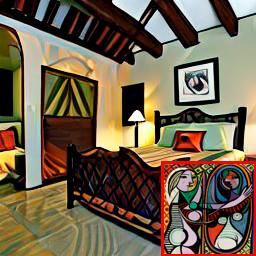} &
            \includegraphics[trim=0 0 0 0,clip,width=0.2\columnwidth]{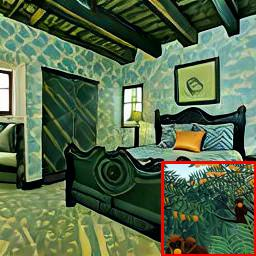} &
            \includegraphics[trim=0 0 0 0,clip,width=0.2\columnwidth]{supp/supp_qualitatives/od_global/images/bed/093.jpg} \\

            \includegraphics[trim=0 0 0 0,clip,width=0.2\columnwidth]{supp/supp_qualitatives/od_global/images/bed/228_original.jpg} &
            \includegraphics[trim=0 0 0 0,clip,width=0.2\columnwidth]{supp/supp_qualitatives/od_global/images/bed/228.jpg} &
            \includegraphics[trim=0 0 0 0,clip,width=0.2\columnwidth]{supp/supp_qualitatives/od_global/images/bed/232.jpg} &
            \includegraphics[trim=0 0 0 0,clip,width=0.2\columnwidth]{supp/supp_qualitatives/od_global/images/bed/234.jpg} &
            \includegraphics[trim=0 0 0 0,clip,width=0.2\columnwidth]{supp/supp_qualitatives/od_global/images/bed/240.jpg} &
            \includegraphics[trim=0 0 0 0,clip,width=0.2\columnwidth]{supp/supp_qualitatives/od_global/images/bed/245.jpg} \\

            \includegraphics[trim=0 0 0 0,clip,width=0.2\columnwidth]{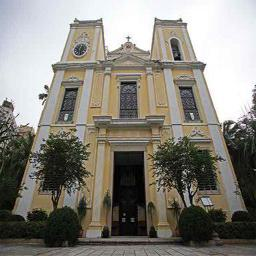} &
            \includegraphics[trim=0 0 0 0,clip,width=0.2\columnwidth]{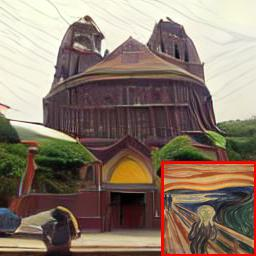} &
            \includegraphics[trim=0 0 0 0,clip,width=0.2\columnwidth]{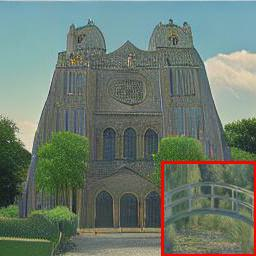} &
            \includegraphics[trim=0 0 0 0,clip,width=0.2\columnwidth]{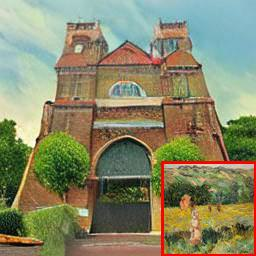} &
            \includegraphics[trim=0 0 0 0,clip,width=0.2\columnwidth]{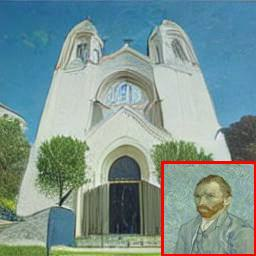} &
            \includegraphics[trim=0 0 0 0,clip,width=0.2\columnwidth]{supp/supp_qualitatives/od_global/images/church/037.jpg} \\

            \includegraphics[trim=0 0 0 0,clip,width=0.2\columnwidth]{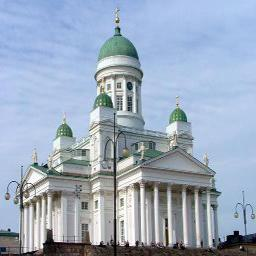} &
            \includegraphics[trim=0 0 0 0,clip,width=0.2\columnwidth]{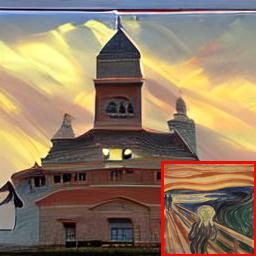} &
            \includegraphics[trim=0 0 0 0,clip,width=0.2\columnwidth]{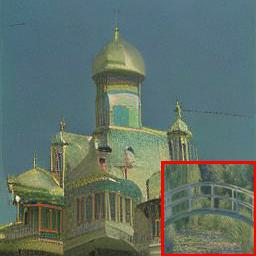} &
            \includegraphics[trim=0 0 0 0,clip,width=0.2\columnwidth]{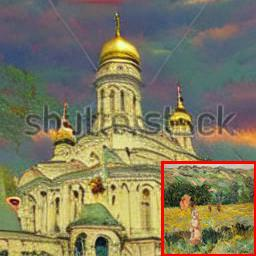} &
            \includegraphics[trim=0 0 0 0,clip,width=0.2\columnwidth]{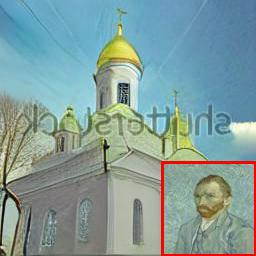} &
            \includegraphics[trim=0 0 0 0,clip,width=0.2\columnwidth]{supp/supp_qualitatives/od_global/images/church/075.jpg} \\

            \includegraphics[trim=0 0 0 0,clip,width=0.2\columnwidth]{supp/supp_qualitatives/od_global/images/church/612_original.jpg} &
            \includegraphics[trim=0 0 0 0,clip,width=0.2\columnwidth]{supp/supp_qualitatives/od_global/images/church/612.jpg} &
            \includegraphics[trim=0 0 0 0,clip,width=0.2\columnwidth]{supp/supp_qualitatives/od_global/images/church/616.jpg} &
            \includegraphics[trim=0 0 0 0,clip,width=0.2\columnwidth]{supp/supp_qualitatives/od_global/images/church/618.jpg} &
            \includegraphics[trim=0 0 0 0,clip,width=0.2\columnwidth]{supp/supp_qualitatives/od_global/images/church/623.jpg} &
            \includegraphics[trim=0 0 0 0,clip,width=0.2\columnwidth]{supp/supp_qualitatives/od_global/images/church/626.jpg} \\

    \end{tabular}
    }
    \captionof{figure}{Visual results for out of domain global appearance manipulation.}
    \label{fig:od_global_supp}
\end{table*}
