# Supplementary material for: PAIR-Diffusion: A Comprehensive Multimodal Object-Level Image Editor
Source: arXiv:2303.17546 source file (2024-04-08)
Supplement: Supplementary file 2 [file od_local.tex]

\begin{table*}
    \centering
    
    \footnotesize
    %\resizebox{\linewidth}{!}{
    \setlength\tabcolsep{0.2pt}
    \begin{tabular}{ccccc}
            Input & \multicolumn{2}{c}{Wall} & \multicolumn{2}{c}{Bed} \\
            \includegraphics[trim=0 0 0 0,clip,width=0.2\columnwidth]{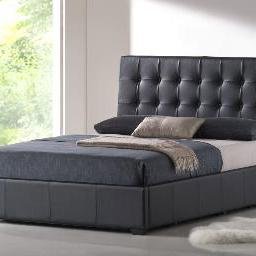} &
            \includegraphics[trim=0 0 0 0,clip,width=0.2\columnwidth]{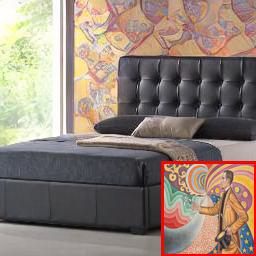} &
            \includegraphics[trim=0 0 0 0,clip,width=0.2\columnwidth]{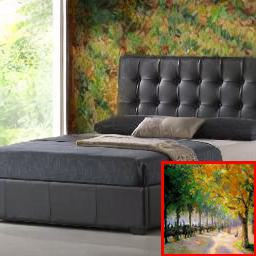} &
            \includegraphics[trim=0 0 0 0,clip,width=0.2\columnwidth]{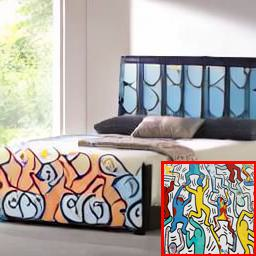} &
            \includegraphics[trim=0 0 0 0,clip,width=0.2\columnwidth]{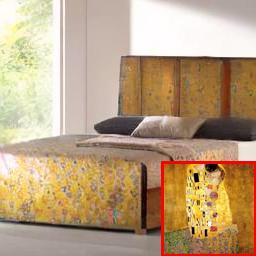} \\
            
            \includegraphics[trim=0 0 0 0,clip,width=0.2\columnwidth]{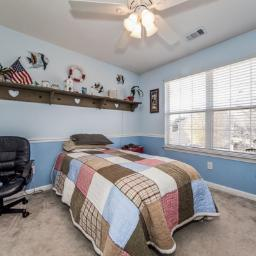} &
            \includegraphics[trim=0 0 0 0,clip,width=0.2\columnwidth]{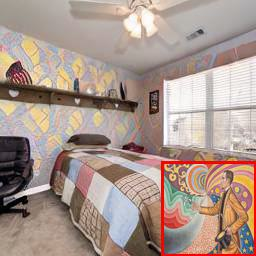} &
            \includegraphics[trim=0 0 0 0,clip,width=0.2\columnwidth]{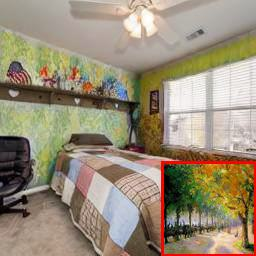} &
            \includegraphics[trim=0 0 0 0,clip,width=0.2\columnwidth]{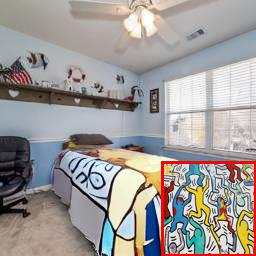} &
            \includegraphics[trim=0 0 0 0,clip,width=0.2\columnwidth]{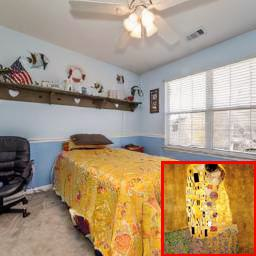} \\

            \includegraphics[trim=0 0 0 0,clip,width=0.2\columnwidth]{supp/supp_qualitatives/od_local/images/bed/210_original.jpg} &
            \includegraphics[trim=0 0 0 0,clip,width=0.2\columnwidth]{supp/supp_qualitatives/od_local/images/bed/134.jpg} &
            \includegraphics[trim=0 0 0 0,clip,width=0.2\columnwidth]{supp/supp_qualitatives/od_local/images/bed/144.jpg} &
            \includegraphics[trim=0 0 0 0,clip,width=0.2\columnwidth]{supp/supp_qualitatives/od_local/images/bed/142.jpg} &
            \includegraphics[trim=0 0 0 0,clip,width=0.2\columnwidth]{supp/supp_qualitatives/od_local/images/bed/138.jpg} \\
            
            Input & \multicolumn{2}{c}{Church} & \multicolumn{2}{c}{Sky} \\
            \includegraphics[trim=0 0 0 0,clip,width=0.2\columnwidth]{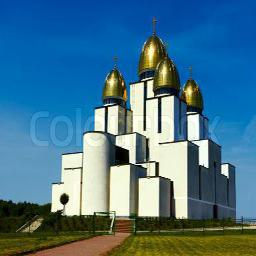} &
            \includegraphics[trim=0 0 0 0,clip,width=0.2\columnwidth]{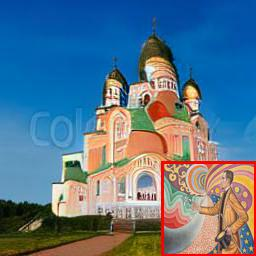} &
            \includegraphics[trim=0 0 0 0,clip,width=0.2\columnwidth]{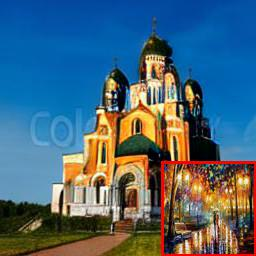} &            \includegraphics[trim=0 0 0 0,clip,width=0.2\columnwidth]{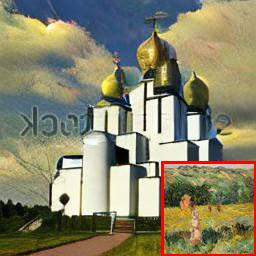} &            \includegraphics[trim=0 0 0 0,clip,width=0.2\columnwidth]{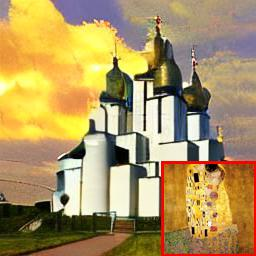} \\

            \includegraphics[trim=0 0 0 0,clip,width=0.2\columnwidth]{supp/supp_qualitatives/od_local/images/church/153_original.jpg} &
            \includegraphics[trim=0 0 0 0,clip,width=0.2\columnwidth]{supp/supp_qualitatives/od_local/images/church/153.jpg} &
            \includegraphics[trim=0 0 0 0,clip,width=0.2\columnwidth]{supp/supp_qualitatives/od_local/images/church/168.jpg} &            \includegraphics[trim=0 0 0 0,clip,width=0.2\columnwidth]{supp/supp_qualitatives/od_local/images/church/163.jpg} &            \includegraphics[trim=0 0 0 0,clip,width=0.2\columnwidth]{supp/supp_qualitatives/od_local/images/church/157.jpg} \\

            \includegraphics[trim=0 0 0 0,clip,width=0.2\columnwidth]{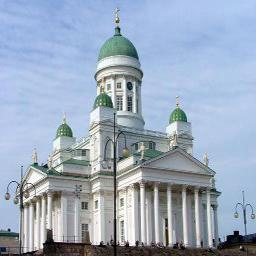} &
            \includegraphics[trim=0 0 0 0,clip,width=0.2\columnwidth]{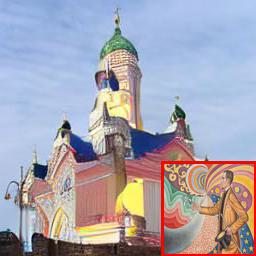} &
            \includegraphics[trim=0 0 0 0,clip,width=0.2\columnwidth]{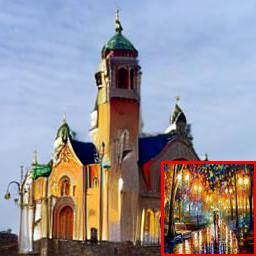} &            \includegraphics[trim=0 0 0 0,clip,width=0.2\columnwidth]{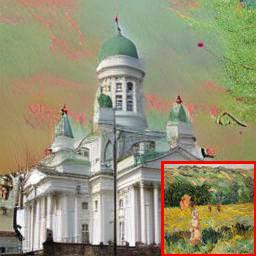} &            \includegraphics[trim=0 0 0 0,clip,width=0.2\columnwidth]{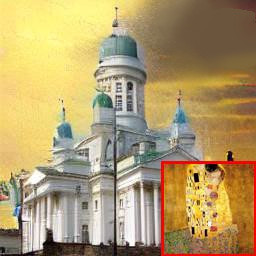} \\
            
    \end{tabular}
    %}
    \captionof{figure}{Visual results for out of domain local appearance manipulation.}
    \label{fig:local_od_apperance_supp}
\end{table*}
